# Supplementary material for: How Knowledge Graph and Attention Help? A Quantitative Analysis into Bag-level Relation Extraction
Source: arXiv:2107.12064 source file (2021-07-26)
Supplement: Supplementary file 1 [file appendix.tex]

\begin{table*}[htbp]
\centering
\begin{tabular}{c|c|c|c|c}

\textbf{Model} & \textbf{AUC}& \textbf{AAcc}& \textbf{AUCV}&\textbf{AUCN} \\ \hline
BRE+ATT &0.878& 0.881&0.941&0.434 \\
$\text{BRE+ATT}_{\text{no pretrain}}$ &0.539&0.798&0.622&0.236\\
BRE+KA  &0.932& 0.857&0.936&0.560  \\
BRE+$\text{KA}_{\text{no pretrain}}$&0.600&0.679&0.867&0.171 \\
BRE+$\text{KA}_{\text{rand}}$ &0.915&0.762&0.936&0.659\\
\hline
\hline
BRE  &0.910& NA&0.932&0.850  \\
$\text{BRE}_{\text{no pretrain}}$ &0.706&NA&0.724&0.617\\
\hline
\hline
BRE+KG  &0.915& NA&0.935&0.856  \\
$\text{BRE+KG}_{\text{no pretrain}}$ &0.773&NA&0.792&0.706\\
$\text{BRE+KG}_{\text{rand}}$ &0.916&NA&0.937&0.846\\
\hline
\hline
SeG  &0.914& NA&0.929&0.759  \\

\end{tabular}
\caption{Test results of models trained on the BagRel-Wiki73K's mix train set. The AUC is the area under the precison-recall curve, AUC w/o noise is computed on the test set whose noisy sentences are all removed, AUC only noise is computed by removing all valid sentences from the test set. For naive models without attention mechanism and SeG, the attention accuracy is NA.}
\label{fewrel-mix}
\end{table*}

\begin{table*}[htbp]
\centering
\begin{tabular}{c|c|c|c|c}

\textbf{Model-Set} & \textbf{AUC}& \textbf{attention acc}& \textbf{AUC w/o noise}&\textbf{AUC only noise} \\ \hline
ATT-mix &0.878& 0.881&0.941&0.434 \\
ATT-half &0.897&0.751&0.932&0.711\\
ATT-pure &0.896&0.713&0.925&0.759\\
\hline
\hline
KG-ATT-mix  &0.932& 0.857&0.936&0.560  \\
KG-ATT-half &0.924&0.720&0.928&0.723\\
KG-ATT-pure & 0.913 &0.617&0.916&0.761\\
\hline
\hline
naive-mix  &0.910& NA&0.932&0.850  \\
naive-half &0.911&NA&0.933&0.847   \\
naive-pure &0.910&NA&0.934&0.841   \\
\hline
\hline
KG-naive-mix  &0.915& NA&0.935&0.856  \\
KG-naive-half &0.919&NA&0.939&0.849   \\
KG-naive-pure &0.918&NA&0.941&0.845   \\
\hline
\hline
SeG-mix  &0.914& NA&0.929&0.759  \\
SeG-half &0.907&NA&0.926&0.775   \\
SeG-pure &0.902&NA&0.921&0.793   \\
\end{tabular}
\caption{Test results of models trained on BagRel-Wiki73K's mix, half mix half pure (half) and pure train set. The result in a row named as X-Y is generated by the model X trained on the Y train set.}
\label{fewrel-3sets}
\end{table*}
